# Supplementary material for: Differential Privacy Meets Neural Network Pruning
Source: arXiv:2303.04612 source file (2023-03-08)
Supplement: Supplementary file 1 [file appendix.tex]

\subsection{Pre-training a classifier using public data}
As a first step of our algorithm, we pre-train a classifier using public data. When choosing which dataset to use for pre-training, it is important to consider that the distribution of the public data should be \textit{similar} to that of the private data.

% pre-training with the public data suffices and the resulting classifier would perform perfectly on the private data. 
%
Second, we consider the case when the gap between two distributions is large. In this case, transferring the knowledge of the learned features from the public data to perform a classification task on the private data gets less useful
% , as the performance of transfer learning with larger domain gaps gets worse
\citep{CVPR_Sparse}. 
What's helpful in this case is that
% In practical scenarios, it is often the case that there is simply no public data that are similar to the private data at hand. 
using more complex data as public data than the private data is useful, as it is easier to simplify complex features by fine-tuning than the other way around. In other words, 
it is useful for the public data to contain the features that are the superset of the features present in the private data. 
For instance, fine-tuning a model for MNIST, which was trained on SVHN, is an easier task than fine-tuning a model for SVHN, which was trained on MNIST, as in this case, the model has to learn entirely new features that were not present in the pre-training phase.

% Third, we consider the scenario of using synthetic datasets that are generated with differential privacy. Among many existing techniques in the literature such as \citep{dpmerf, sinkhorn_21, gs-wgan},
% we use a recent work \citep{dpmepf} which can generate synthetic data for a complex dataset like CIFAR-10  at a reasonable privacy level ($\epsilon \approx 2\%$) to test this scenario. In this case, however, we split some part of privacy budget to generate the synthetic data with which we can pre-train the network; then use the rest of the privacy budget for fine-tuning the model with our method. 

Structured vs unstructured pruning

%Given pruning rate $p$ we sort each layer according to the magnitude. The bottom $p\%$ parameters are frozen, that is their weights remain unchanged in further steps.
and 
\textit{(ii) structured pruning} \citep{ifantis1991bounds, louizos2017bayesian, oh2019radial, adamczewski21a} removes the entire computational unit such as channels in convolutional layers or neurons in fully connected layers based on each unit's importance whose definition varies method by method. Unlike unstructured pruning, structured pruning provides practical acceleration by reducing the memory requirement and increasing the speed during inference. However, in our case, since we are not bound by creating a smaller model, we focus on unstructured pruning which does not impose any structural constraints on the choice of dropped parameters and focuses on helping improve the privacy and accuracy trade-off.
